# Supplementary material for: Quantifying Membership Inference Risks in Genomic Data Sharing: The Role of Attacker's Auxiliary Information
Source: arXiv:2611.18909 source file (2026-11-13)
Supplement: Supplementary file 1 [file Appendix_A.tex]

\newpage
\begin{appendices}
\section{Appendix A: Formal Proofs}
\label{app:proofs}

\subsection*{Proof of Proposition~\ref{prop:sensitivity}
($\ell_1$ Sensitivity of PCA Scores)}

Let $\mathbf{V} \in \mathbb{R}^{p \times d}$ be a fixed loading matrix with
unit-norm columns $\|\mathbf{v}_j\|_2 = 1$ for all $j \in \{1,\ldots,d\}$.
Let $\mathbf{x}_i, \mathbf{x}_i' \in [0,1]^p$ be two neighboring normalized
genotype vectors differing in at most one individual's record. The difference
in PCA scores is:
\[
\mathbf{y}_i - \mathbf{y}_i' = (\mathbf{x}_i - \mathbf{x}_i')\mathbf{V}_{1:d}.
\]
Applying the $\ell_1$ norm:
\begin{align*}
\|\mathbf{y}_i - \mathbf{y}_i'\|_1
&= \sum_{j=1}^{d} \bigl|(\mathbf{x}_i - \mathbf{x}_i')^\top \mathbf{v}_j\bigr| \\
&\leq \sum_{j=1}^{d} \|\mathbf{x}_i - \mathbf{x}_i'\|_2 \cdot \|\mathbf{v}_j\|_2
  \quad \text{(Cauchy-Schwarz)} \\
&= d \cdot \|\mathbf{x}_i - \mathbf{x}_i'\|_2.
\end{align*}
Since SNP values are normalized to $[0,1]$ and a single record change affects
at most $p$ coordinates by at most~1, applying Cauchy-Schwarz with the
$\ell_0$ norm bound gives $\|\mathbf{x}_i - \mathbf{x}_i'\|_2 \leq \sqrt{2}$
(at most two non-zero entries per SNP change under diploid encoding, each
bounded by~1). Substituting:
\[
\|\mathbf{y}_i - \mathbf{y}_i'\|_1 \leq d\sqrt{2} \leq 2\sqrt{d}
\quad \text{for } d \geq 1.
\]
The sensitivity is therefore $s = 2\sqrt{d}$, and the Laplace noise scale is
$\lambda = s/\epsilon = 2\sqrt{d}/\epsilon$. \hfill$\square$

\subsection*{Proof of Proposition~\ref{prop:leakage} (Server Leakage Bound)}

The server reconstructs $\hat{\mathbf{x}}_i = \tilde{\mathbf{y}}_i \cdot
\mathbf{V}^{\dagger} + \boldsymbol{\mu}$, where
$\tilde{\mathbf{y}}_i = \mathbf{y}_i + \boldsymbol{\eta}$ and
$\boldsymbol{\eta} \sim \text{Lap}(\lambda)^d$. The reconstruction error is:
\[
\|\hat{\mathbf{x}}_i - \mathbf{x}_i\|_2
= \|\boldsymbol{\eta}\mathbf{V}^{\dagger}\|_2.
\]
Since $\mathbf{V}$ has unit-norm columns, $\|\mathbf{V}^{\dagger}\|_F \geq
\sqrt{d}$. Therefore:
\[
\mathbb{E}\bigl[\|\boldsymbol{\eta}\mathbf{V}^{\dagger}\|_2\bigr]
\geq \mathbb{E}\bigl[\|\boldsymbol{\eta}\|_2\bigr]
= \sqrt{d} \cdot \mathbb{E}[|\eta_1|]
= \sqrt{d} \cdot \lambda
= \sqrt{d} \cdot \frac{2\sqrt{d}}{\epsilon}
= \frac{2d}{\epsilon}.
\]
For $\epsilon=1$ and $d=2$: expected reconstruction error $\geq 4$, which
exceeds the maximum normalized SNP variation of~2. \hfill$\square$.
\end{appendices}
