# Supplementary material for: Quantifying Membership Inference Risks in Genomic Data Sharing: The Role of Attacker's Auxiliary Information
Source: arXiv:2611.18909 source file (2026-11-13)
Supplement: Supplementary file 2 [file Appendix_B.tex]

\newpage
\begin{appendices}
\section{Metric Definitions}
\label{app:metrics}

\textbf{MIA Power} at false-positive rate $\alpha$: Let $T$ be set so that
$\alpha$ of the control group falls below $T$ in minimum Euclidean distance
to $\tilde{D}_R$. Power is the fraction of the target group $H \subset D_R$
satisfying $\min_{u \in \tilde{D}_R} \|\mathbf{v} - \mathbf{u}\|_2 \leq T$.

\textbf{Precision}: Of the individuals flagged as members (distance $\leq T$),
the fraction that are true members.

\textbf{Recall}: Of the true members, the fraction correctly flagged
(distance $\leq T$).

\textbf{U-ReRo}~\cite{Guerra2024Analysis}: $|P_{\text{member}} - P_{\text{nonmember}}|$
where each quantity is the fraction of the respective group achieving
reconstruction error $\leq \eta = 0.5$ under the pseudoinverse reconstruction
defined in evaluation section.

\section{Genomic Background }
The human genome is the complete set of human DNA, composed of four nucleotides: adenine (A), guanine (G), cytosine (C), and thymine (T). It comprises 23 pairs of chromosomes, more than 20,000 genes, and roughly 3 billion base pairs. DNA serves as the blueprint for development, guiding the progression from a single cell to a full organism, while genes contribute to individual traits. An allele is a variant of a DNA sequence at a specific chromosomal location, typically a single nucleotide (though sometimes a short segment). Most of the genome is shared across individuals, but a small fraction varies, producing genetic variation. The most common form is the single nucleotide polymorphism (SNP), a key marker for linking genes to diseases. Most SNPs are biallelic, with a major allele (more frequent) and a minor allele (less frequent). In this work, SNPs are encoded as 0, 1, or 2 based on the number of minor alleles present.

\section{Related Work}\label{sec:Related_works}
The sharing of genomic data has accelerated biomedical research but has also introduced substantial privacy challenges, especially from MIAs, which attempt to infer whether an individual appears in a shared dataset. Prior work has proposed defenses that balance privacy and utility from multiple angles.

\textbf{Statistical Approaches to Privacy Risks:}
In \cite{Homer2008Resolving}, a statistical test showed that individuals can be detected in aggregate genomic datasets by comparing to external high-density genotype data, including inferring case/control membership in GWAS. This result helped motivate moving some GWAS outputs from open to controlled access, underscoring the need for privacy safeguards in genomic data sharing.

\textbf{Differential Privacy in Genomic Data:}
Differential privacy (DP) is a widely used framework for protecting sensitive data. \cite{chen2021Differential} studied DP defenses against MIAs for genomic ML models, finding that stronger privacy (smaller $\epsilon$) reduces accuracy in a roughly log-like manner and that sparsity/regularization can further reduce MIA vulnerability in high-dimensional settings.
In \cite{Sarathy2011Evaluating}, the authors analyzed Laplace noise for numeric datasets, highlighting utility--privacy trade-offs: in large datasets, Laplace noise may be insufficient for protection, while in small datasets the required noise can severely harm utility; they also note difficulties for skewed or unbounded data.
Building on DP for genomics, \cite{Yilmaz2022Genomic} proposed dependent local DP methods that exploit genomic correlations to improve utility while preserving privacy.

\textbf{Game-Theoretic and Statistical Modeling Approaches:}
\cite{zhang2024bayesnash} modeled publisher--adversary interactions as a Bayesian game, characterizing strategic noise addition that mitigates risk while maintaining utility.
In \cite{Halimi2022Privacy}, likelihood ratio tests (LRT) were used to quantify membership risk from shared minor allele frequencies (MAFs), providing a practical benchmark for evaluating privacy mechanisms.

\textbf{Vulnerabilities in Different Genomic Data Types:}
\cite{humbert2017Quantifying} showed that sharing familial SNP data can amplify privacy loss: adversaries can leverage kinship correlations and auxiliary sources (e.g., public genomes) to infer an individual’s genome even from partial disclosures.
\cite{Bu2021Haplotype} demonstrated stronger membership inference using haplotypes, achieving high power without needing the target’s genome and enabling reconstruction of rare, distinctive haplotypes from summary information—highlighting risks even for seemingly minimal releases.

\textbf{Metrics and Evaluation of Privacy Mechanisms:}
In \cite{Guerra2024Analysis}, Unbiased Reconstruction Robustness (U-ReRo) was introduced to reduce bias in DP evaluations and assess whether protections are membership-neutral for members and non-members.

\textbf{Broader Context and Future Directions:}
\cite{Hu2022Membership} surveyed MIAs more broadly and emphasized that defenses should be tailored to the data type and threat model—an especially relevant principle for genomic settings.

Together, these studies motivate privacy mechanisms that account for realistic auxiliary information and dataset structure. Our work builds on this foundation by evaluating MIA risk across practical scenarios, incorporating U-ReRo, and using PCA-based spatial analysis to better understand how dataset proximity shapes privacy risk.

\end{appendices}
